# Supplementary material for: Real space lensing reconstruction using cosmic microwave background polarization
Source: arXiv:1709.02227 source file (2017-09-07)
Supplement: Supplementary file 1 [file appendix_plot_comments.tex]

\section{KM: Commentary on plots}

\subsection{General notes placed here}

\begin{enumerate}
 
\item Discuss applications that had in mind? more info since less tapering of map, go to lower ell on small patches, consistency checks, large-scale shear vs conv for Planck - systematics or dA fluctuations, + Other?
\item Why use maps to evaluate reconstructions, not power spectra? Need higher SN to see map modes vs ps modes - this is a more stringent requirement; Need to correct for multiplicative bias to get ps shape correct - best to wait for extended estimator with no multiplicative bias in forthcoming paper; Need to correct for additive bias in ps estimation - defer to future work.

\end{enumerate}
